# Supplementary material for: Mining Error Templates for Grammatical Error Correction
Source: arXiv:2206.11569 source file (2022-06-23)
Supplement: Supplementary file 1 [file appendix.tex]

\section{Examples of Search Patterns}
\input{tables/search_pattern}
\label{sec:ap}
